# Supplementary material for: Minimum Overhead Beamforming and Resource Allocation in D2D Edge Networks
Source: arXiv:2007.12963 source file (2022-08-16)
Supplement: Supplementary file 1 [file appendixNotused.tex]

\section{Proof of Lemma 1}
\label{sec:appLem}

\begin{proof}
    The optimal solution ${{\bf{z}}_{k',{i}}^* }$ and ${w_k^*} $ to maximize ${h_k}(\{ {{\bf{g}}_k}\} ,{{\bf{z}}_{k',{i}}},{w_k})$ are given by \eqref{eq:optsol:z} and \eqref{eq:optsol:w} where $h_k$ is given in \eqref{eq:h}. Therefore, the right hand side of \eqref{eq:Rh} is given by
\begin{align}
    & \mathop {\max }\limits_{{{\bf{z}}_{k',{i}}},{w_k}} 
    {h_k}(\{ {{\bf{g}}_k}\} ,{{\bf{z}}_{k',{i}}},{w_k})  
    \\
    & \hspace{0.8cm}=
    {h_k}(\{ {{\bf{g}}_k}\} ,{{\bf{z}}_{k',{i}}^* },{w_k^*})
    \\
    & \hspace{0.8cm}= 
    - ({w_k^*})^{ - 1} e_k^{{\rm{mse}}}(  \{ {{\bf{g}}_k}\} ,{{\bf{z}}_{k',{i}}^* }  ) - \log {w_k^*} + 1
    \\
    & \hspace{0.8cm}= 
    -\log \big( { e_k^{{\rm{mse}}}(  \{ {{\bf{g}}_k}\} ,{{\bf{z}}_{k',{i}}^* } )} \big)
\end{align}
%{h_k}(\{ {{\bf{g}}_k}\} ,{{\bf{z}}_{k',{i}}},{w_k}) =  - w_k^{ - 1} e_k^{{\rm{mse}}}(  \{ {{\bf{g}}_k}\} ,{{\bf{z}}_{k'{i}}}  ) - \log {w_k} + 1.
%    \label{eq:h}
Then, we remain proving the following.
\begin{equation}
    R_{k,k'} = -\log \big( { e_k^{{\rm{mse}}}(  \{ {{\bf{g}}_k}\} ,{{\bf{z}}_{k',{i}}^* } )} \big).
\end{equation}
Since this is the well-known relationship between the
rate and the mean-square-error (MSE) given the minimum MSE (MMSE) receiver, which is proved in many works, e.g., \cite{Qingjiangshi}, we omit to prove the  remaining relation.
\end{proof}
